# Supplementary material for: On The Empirical Effectiveness of Unrealistic Adversarial Hardening Against Realistic Adversarial Attacks
Source: arXiv:2202.03277 source file (2023-05-22)
Supplement: Supplementary file 1 [file 10-supplementary-old.tex]

\newpage
\section{Appendix}

\subsection{}


\begin{table}[ht!]
\centering
\caption{Statistical values of input lengths for  datasets used during adversarial fine-tuning in text classification use case}
\begin{tabular}{lllll} 
\toprule
Dataset               & Mean        & Std         & Min & Max  \\ 
\hline
Rotten Tomatoes~      & 18.49~ ~ ~~ & 8.58~ ~ ~~  & 1   & 51   \\
Tweet Offensive & 22.12~ ~ ~~ & 15.21~ ~ ~~ & 2   & 104  \\
AG News               & 38.78~ ~ ~~ & 11.18~ ~ ~~ & 11  & 178  \\
\bottomrule
\end{tabular}
\label{tab-text_dataset_char}
\end{table}


\begin{figure}[ht!]
    \begin{subfigure}{\linewidth}
  \includegraphics[width=\linewidth]{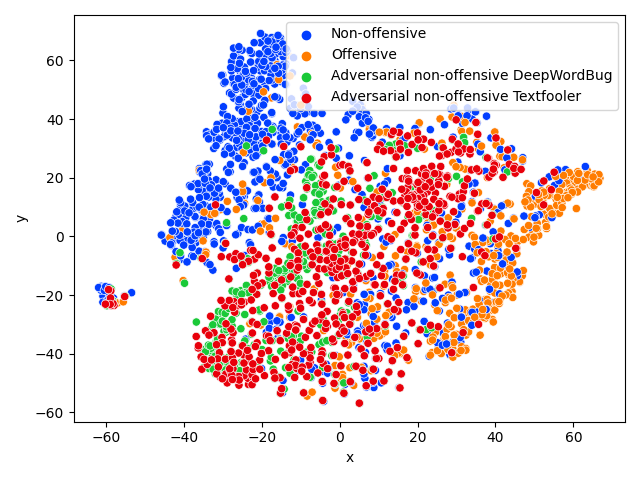}
    \caption{TweetEval (Offensive) non-offensive tweets}
  \end{subfigure}\hfill
  \begin{subfigure}{\linewidth}
  \includegraphics[width=\linewidth]{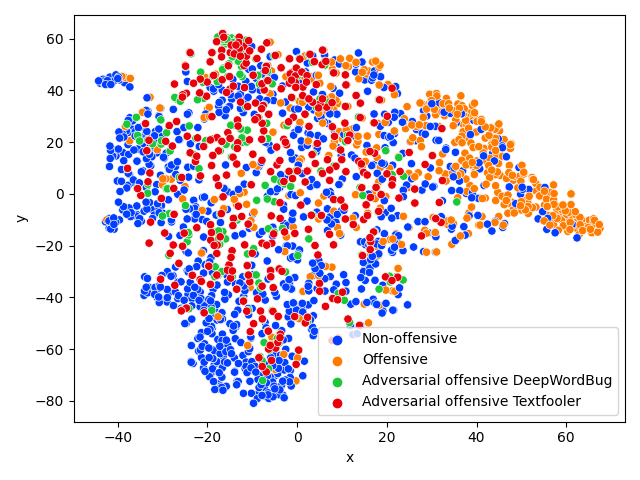}
    \caption{TweetEval (Offensive) offensive tweets}
  \end{subfigure}\hfill
  \caption{t-SNE sentence embeddings from the last layer latent representation of the models. The graphs include the original examples and the successful adversarial examples generated by DeepWordBug and TextFooler}
  \label{fig-text-rq3-supp}
  \end{figure}






\subsection{Evaluation of the hardening strategies on different classes of Text Classification task}
\label{sec:appendix-text}


\paragraph{\textbf{Impact of the hardening on each class}}

We first investigate whether constrained and unconstrained attacks impact in a same manner the positive and negative classes. We provide the improvements of each hardening strategy for each dataset in Table \ref{tab-acc-class-apx} for the positive classes (positive reviews and offensive tweets) and  for the negative classes(negative reviews and non-offensive tweets). 


\begin{table}[ht!]
\centering
\caption{Accuracy of clean and adversarially fine-tuned models for each class (in \%). DeepWordBug is noted with DWB and TextFooler with TF}
\label{tab-acc-class-apx}
\begin{tabular}{llllll} 
\toprule
Dataset   & Trained & Class         & DWB    & TF             & $\Delta$ TF  \\
          & against &               &        &                &              \\ 
\midrule
Rottten~  & Clean   & Negative      & 38.88  & 8.54           &              \\
Tomatoes  &         & Positive      & 0.22   & 2.46           &              \\
          & DWB     & Negative      & 31.9~  & 14.25~         & +5.71        \\
          &         & Positive      & 25.5~  & 4.47\textbf{~} & +2.01        \\
          & TF      & Negative      & 43.1   & 23.57~         & +15.03       \\
          &         & Positive      & 12.1~  & 12.1~          & +9.64        \\
Tweet~    & Clean   & Non-offensive & 35.31  & 16.31          &              \\
Offensive &         & Offensive     & 0.6    & 0.91           &              \\
          & DWB     & Non-offensive & 80.06~ & 27.58~         & +11.27       \\
          &         & Offensive     & 0~     & 0.32~          & -0.59        \\
          & TF      & Non-offensive & 72.6   & 56.57~         & +40.26       \\
          &         & Offensive     & 0~     & 0.4~           & -0.51        \\
\bottomrule
\end{tabular}
\end{table}

For Rotten Tomatoes, initially, the clean model is less robust on the positive reviews when evaluated both in DeepWordBug and TextFooler adversarial sentences. However, both the positive and negative classes benefit similarly from the adversarial fine-tuning using both the unconstrained (DeepWordBug) and constrained (TextFooler) attacks. With TextFooler, the positive class gains 9.64\% robust accuracy and the negative classes gain 15.03\%.

For Tweet Offensive dataset, initially, the clean model is very vulnerable on offensive class. It achieves only 0.60\% accuracy when evaluated with DeepWordBug and 0.91\% with TextFooler. Fine-tunning with DeepWordBug or TextFooler does not help the robustness in this class. However, the non-offensive class benefits of a major improvement on robustness, especially when fine-tunned with TextFooler (+40.26\%).
One reason might be that the pool of offensive words is small and once the model learns to include them in non-offensive sentences during fine-tuning, it is able to later recognize the adversarial sentences as non-offensive and this increases the robustness for the positive class.

%In RQ1 and RQ2 we were interested on the general improvement of robustness. However, from image domain we know that not all classes behave similarly during model hardening. Therefore, we study the robustness of the two classes separately. The results are given in Table \ref{tab-acc-class}


%The first observation that we have from the table is that for RottenTomatoes the robust accuracy we saw in RQ1 comes almost evenly distributed for both classes. However, for Tweet Offensive, in clean model the offensive class is not robust at all (only 0.9\% accuracy). Fine-tunning the model does not help on increasing the robustness for this class, it is actually slightly worse (-0.59\% for DeepWordBug and -0.51\% for TextFooler). However, the non-offensive class benefits of a major improvement on robustness, especially when fine-tunned with TextFooler (+40.26\%).  One reason might be that the pool of offensive words is small and once the model learns to include them in non-offensive sentences during fine-tuning, it is able to later recognize the adversarial sentences as non-offensive.

\textbf{Classes are not equally robust to the attacks and profit differently from the hardening process. The overall increase in robustness may actually only favour one class.}

% The results given in Table \ref{tab-acc-class-apx} show the clean model for Rotten Tomatoes dataset is more robust on negative class for both DeepWordBug and TextFooler.  Similarly, for Tweet Offensive  the model is more robust  in non-offensive class. For both datasets, fine-tunning with DeepWordBug  gives a better improvement in robust accuracy when evaluating with TextFooler for the  negative  (+5.71) and non-offensive class (+11.27). As a reminder we are interested on the robustification against TextFooler as the more realistic attack. Fine-tunning with TextFooler, provides a better boost in accuracy for the same classes, respectively negative (+15.03) and non-offensive class (40.26\%). 

% \textbf{The results show that the classes that are already more robust, benefit most from the hardening process}

We investigate next how the robustness towards one or another attack affects the hardening process for each class. From the Table \ref{tab-acc-class-apx}, the clean model is less robust against DeepWordBug for positive reviews and offensive tweets. However, the difference with TextFooler is not significant, respectively only 2.24\% and 0.3\%. Fine-tuning with DeepWordBug in the first dataset does not give a higher improvement in robust accuracy compared to TextFooler (2.01\% vs 9.64\%). In the second dataset, there is a decrease in robust accuracy of -0.59\%, which is very similar to -0.51\% by TextFooler. From Table \ref{tab-acc-class-apx} we see that  the clean model is less robust to TextFooler than DeepWordBug for negative reviews and non-offensive tweets class. Fine-tuning with TextFooler improves the robust accuracy for these classes with respectively  +15.03\%  and +40.26\%. This is a higher boost that the one gained from fine-tuning with DeepWordBug ( +5.71 \% for negative reviews and +11.27\% for non-offensive tweets)

 
\textbf{Classes that are less robust against TextFooler compared to DeepWordBug, benefit more when the model is fine-tuned with TextFooler rather than DeepWordBug}

%\textbf{The class where the adversarial examples fall closer to the initial sentences are more robust, and the vice-versa.}





% \begin{figure*}[ht!]
%   \begin{subfigure}{0.45\linewidth}
%   \includegraphics[width=\linewidth]{figures/rotten_tomatoes_clean_both_embd_class_0.png}
%     \caption{Rotten Tomatoes negative reviews}
%   \end{subfigure}\hfill
%     \begin{subfigure}{0.45\linewidth}
%   \includegraphics[width=\linewidth]{figures/rotten_tomatoes_clean_both_embd_class_1.png}
%     \caption{Rotten Tomatoes positive reviews}
%   \end{subfigure}\hfill
%     \begin{subfigure}{0.45\linewidth}
%   \includegraphics[width=\linewidth]{figures/tweet_eval_clean_both_embd_class_0.png}
%     \caption{TweetEval (Offensive) non-offensive tweets}
%   \end{subfigure}\hfill
%   \begin{subfigure}{0.45\linewidth}
%   \includegraphics[width=\linewidth]{figures/tweet_eval_clean_both_embd_class_1.png}
%     \caption{TweetEval (Offensive) offensive tweets}
%   \end{subfigure}\hfill
%   \caption{Sentence embeddings of initial inputs and adversarial }
%   \label{fig-text-rq3}
%   \end{figure*}
  
% \begin{figure}[!ht]
%   \includegraphics[width=\linewidth]{figures/rotten_tomatoes_clean_both_embd_class_1.png}
%   \caption{Sentence embeddings of initial inputs and adversarial for positive class in Rotten Tomatoes dataset.}
%   \label{fig-text-rq3}
%   \end{figure}


%The embeddings do not quantify the spread of adversarial examples, hence 
%We present in Table \ref{tab-text-cluster} the quantitative analysis of the clusters.

We observe in Table \ref{tab-text-cluster}
that the class with the lower clustering score between the initial clean sentences and successful adversarial examples, is the most robust class. This holds true both for evaluation  with  DeepWordBug  and TextFooler adversarial sentences in both datasets. For example, for Rotten Tomatoes dataset the robust accuracy of the clean model on negative class (8.54\%) against TextFooler is higher than positive class (2.46\%) (ref Table \ref{tab-acc-class-apx} ). In Table \ref{tab-text-cluster}, we see that the Calinski-Harabasz clustering score between initial sentences and generated adversarial sentences is lower for the negative reviews  (62.61) compared to positive reviews (131.36). Similar observation can be done for the other dataset and other classes. A lower clustering score between the initial sentences and generated adversarial sentences means that the clusters are not well separated. Hence, the adversarial sentence embeddings are close to the initial ones and widely spread. 


\begin{table}
\centering
\caption{Clustering scores for adversarial samples generated by DeepWordBug( noted DWB) and TextFooler(noted TF) for each class. A higher score indicates better clustering for both metrics.}
\label{tab-text-cluster}
\begin{tabular}{lllll} 
\toprule
Dataset                          & Class         & Clusters      & Silhouette & CH      \\ 
\hline
\multirow{6}{*}{Rotten Tomatoes} & Negative      & DWB - TF      & -0.01      & 7.64    \\
                                 &               & Initial - DWB & 0.09       & 42.55   \\
                                 &               & Initial  - TF & 0.08       & 62.61   \\
                                 & Positive      & DWB - TF      & 0.02       & 11.66   \\
                                 &               & Initial - DWB & 0.15       & 171.31  \\
                                 &               & Initial - TF  & 0.12       & 131.36  \\
                                 &               &               &            &         \\
\multirow{6}{*}{Tweet Offensive} & Non-offensive & DWB - TF      & 0          & 23.01   \\
                                 &               & Initial - DWB & 0.04       & 36.78   \\
                                 &               & Initial - TF  & 0.06       & 78.99   \\
                                 & Offensive     & DWB - TF      & 0          & 1.48    \\
                                 &               & Initial - DWB & 0.11       & 94.86   \\
                                 &               & Initial - TF  & 0.09       & 82.95   \\
\bottomrule
\end{tabular}
\end{table}

In Table \ref{tab-text-cluster-diff} we present the relationship between the clustering score and the gap in robust accuracy for DeepWordBug and TextFooler. The results show that a greater gap in robust accuracy from clean models does not necessarily result in better separated adversarial sentence embeddings between TextFooler and DeepWordBug. The greatest robust accuracy gap between TextFooler and DeepWordBug happens for the  negative class in Rotten Tomatoes dataset. However, the best separated clusters of generated sentences between DeepWordBug and TextFooler in Table \ref{tab-text-cluster} is the non-offensive class in Tweet Offensive dataset. 

\textbf{DeepWordBug generates adversarial embeddings with a higher concentration in the embedding space compared to TextFooler. The class where adversarial embeddings of DeepWordBug are better clustered in relation to adversarial embeddings from TextFooler, is not always the  class where the robust accuracy differs the most.} 


\begin{table}[ht!]
\centering
\caption{}
\label{tab-text-cluster-diff}
\begin{tabular}{llll} 
\toprule
Dataset               & Class         & CH Score & $\Delta$ TF,DWB \\ 
\hline
Rotten Tomatoes       & Negative      & 7.64     & -30.34                   \\
                      & Positive      & 11.66    & +2.24                     \\
Tweet Offensive & Non-offensive & 23.01    & -19.00                      \\
                      & Offensive     & 1.48     & +0.30                      \\
\bottomrule
\end{tabular}
\end{table}
